# Supplementary material for: Resilient and Distributed Multi-Robot Visual SLAM: Datasets, Experiments, and Lessons Learned
Source: arXiv:2304.04362 source file (2023-04-10)
Supplement: Supplementary file 1 [file additional_results.tex]

\begin{figure}[!t]
	\centering
	\includegraphics[trim={0 0 0 0},clip, width=1.0\columnwidth]
	{figures/ablations/1207_distributed_alpha-area-plot}
	\caption{{Varying visual similarity threshold ($\alpha$) on \Tunnels dataset}.}\label{fig:ablation_alpha}
\end{figure}

\begin{figure}[!t]
	\centering
	\includegraphics[trim={20 20 20 20},clip, width=1.0\columnwidth]{figures/bandwidth_evolution.pdf}
	\caption{Breakdown of message sizes (in log scale) transmitted over time from one robot to another for the four different communication patterns on the \Hybrid dataset.}\label{fig:bandwidth_evolution}
\end{figure}

\begin{figure}[!t]
	\centering
	\includegraphics[trim={0 0 0 0},clip, width=1.0\columnwidth]{figures/centralized_system.pdf}
	\caption{Centralized base-line system for comparison against distributed.
		Components are implemented to best resemble their fully-distributed counterparts.}\label{fig:centralized}
\end{figure}
